# Supplementary material for: On the Out of Distribution Robustness of Foundation Models in Medical Image Segmentation
Source: arXiv:2311.11096 source file (2023-11-18)
Supplement: Supplementary file 1 [file appendix.tex]

\newcommand\tab[1][5mm]{\hspace*{#1}}
\appendix
\section*{Supplementary Material}
% --------------------------------------
%Ccomment above lines for a separate appendix file
% --------------------------------------
We present below LVM-Med pseudo-code (Section \ref{sec:pseudo-code}), implementations used in downstream tasks (Section \ref{sec:pre-downs-settings}), additional ablation studies of LVM-Med (Section \ref{sec:ablation-lvm-med}), further  prompt-based segmentation results on 3D datasets, image classification benchmark (Section \ref{sec:linear-seg}), predicted masks using the user-based prompt (Section \ref{sec:visualize_images}), and finally the dataset overview (Section \ref{sec:dataset_overview}).   
\section{LVM-Med Pseudo-code}
\label{sec:pseudo-code}
First, we provide a pseudo-code for training LVM-Med in Pytorch style:
\\ \rule{\textwidth}{0.4pt}
\com{\# $\mathtt{f_{\theta}}$:\,encoder network, $\mathtt{h_{\phi}}$:\,projector network, $\mathtt{g_{\epsilon}}$:\,message passing network,}
\\
\com{\# k\_nodes:\,number of nearest neighbors, Avg:\,average pooling, } 
\\ \com{\# pos:\,position of image after transform, cos:\,cosine similarity,}
\\ 
\com{\# $\mathtt{\alpha}$:\,coefficient trades off between global and local costs, $\mathtt{L_2}$:\,L2-distance,  }
\\
\com{\# $\mathtt{\gamma}$:\,maximum pairs are kept, select\_top:\,select to keep the $\mathtt{\gamma}$ best matches.}
\\
\\ \code{for X in loader:}  \com{\# load a batch X = $\mathtt{\left[x_1, x_2,...,x_N\right]}$ with N samples}
\\
\tab \com{\# apply two transformations s and t} 
\\
\tab \code{$\mathtt{X^{s},\ Pos^{s} = s(X)}$} \ \com{\# $\mathtt{X^{k} = \left[x_1^{k},x_2^{k},...,x_{N}^{k}\right]}$,\ $\mathtt{Pos^{k} = \left[pos_{1}^{k}, pos_{2}^{k},...,pos_{N}^{k}\right],\ k \in \{s, t\}}$}\\
\tab \code{$\mathtt{X^{t},\ Pos^{t} = t(X)}$} 
\\
\\
\tab \com{\# compute feature representations}
\\
\tab \code{$\mathtt{Y^{s} = f_{\theta}(X^{s});\ Y^{t} = f_{\theta}(X^{t})}$}  \com{\# feature dimensions:NxDxRxS}
\\
\\
\tab \com{\# applying projection} 
\\
\tab \code{$\mathtt{Z^{s} = h_{\phi}(Avg(Y^{s}));\ Z^{t} = h_{\phi}(Avg(Y^{t}))}$}  \com{\# dimensions:NxF}
\\
\\
\tab \com{\# build graph structures and message passing}
\\
\tab \code{$\mathtt{G^{s}}$ = k-nearest-neighbor($\mathtt{Z^{s}}$, k\_connects)}
\\
\tab \code{$\mathtt{G^{t}}$ = k-nearest-neighbor($\mathtt{Z^{t}}$,k\_connects)}
\\
\tab \code{$\mathtt{\hat{Z}^{s} = g_{\epsilon}(G^{s}, Z^{s})}$;\ $\mathtt{\hat{Z}^{t} = g_{\epsilon}(G^{t}, Z^{t})}$}
\\
\\
\tab \com{\# compute vertex and edge affinity matrices}
\\
\tab \code{$\mathtt{c_{ia}^{v} = \alpha * \,cos(\hat{z}_{i}^{s}, \hat{z}_{a}^{t}) + (1- \alpha)*\,local\_cost(y_{i}^{s},\,y_{a}^{t},\,pos_{i}^{s},\,pos_{a}^{t})}$}\ \com{\# affinity $\mathtt{x_{i}^{s}}$ \& $\mathtt{x_{a}^{t}}$}
\\
\tab \code{$\mathtt{c^{e}_{ia, jb} = cos((\hat{z}_{i}^{s} - \hat{z}_{j}^{s}),(\hat{z}_{a}^{t} - \hat{z}_{b}^{t}))}$}\ \com{\# affinity between edges $\mathtt{v_{ij}^{s}, v_{ab}^{t}}$ }
\\
\tab \code{$\mathtt{c^v = \{c_{ij}^{v}\} \in R^{N\times N};\ c^{e} = \{c^{e}_{ia, jb}\} \in R^{|E^{s}||E^{t}|}}$} \ \com{\# $\mathtt{E^{k}}$ be a set of edges in $\mathtt{G^{k},\,k\in \{s,t\}}$}
\\
\\
\tab \com{\# perturbed costs with Gumbel noise}
\\
\tab \code{$\mathtt{\epsilon, \epsilon' \sim Gumbel(0, 1)}$}
\\
\tab \code{$\mathtt{c^v = c^v + \epsilon;\ c^e = c^e + \epsilon'}$}
\\
\\
\tab \com{\# solving graph matching and compute loss}
\\
\tab \code{$\mathtt{\hat{v} = GM(c^v, c^e)}$}
\\
\tab \code{$\mathtt{L(\hat{\bm{v}}, \bm{v}^*) = \hat{\bm{v}}.(1-\bm{v}^*) + \bm{v}^*.(1-\hat{\bm{v}})}$}
\ \com{\# compute hamming loss}
\\
\\ 
\tab \com{\# update network}
\\ \tab \code{L.backward()}\ \com{\# approximate ($\mathtt{\partial L/\partial c^v, \partial L/\partial c^e}$) by Algorithm 1.}
\\ \tab \code{Update($\mathtt{g_{\epsilon}.params}$),\ Update($\mathtt{h_{\phi}.params}$),\,Update($\mathtt{f_{\theta}.params}$)}
\\
\\
\com{\# define local\_cost}
\\
\code{def local\_cost($\mathtt{y_{i}^{s},\,y_{a}^{t},\,pos_{i}^{s},\,pos_{a}^{t}}$):}
\\ 
\\ \tab \com{\# location-based local cost}
\\ \tab \code{$\mathtt{y_{i,nn}^{s} = torch.zeros\_like(y_{i}^{s})}$}
\\
\tab \code{for r, s in R, S:}
\\
\tab \tab \code{r', s' = argmin($\mathtt{\left(L_2(pos_{i}^{s}[r, s],\ pos_{a}^{t}[r',s']\right)}$)}
\\
\tab \tab \code{$\mathtt{y_{i,nn}^{s}[r, s] = y_{a}^{t}[r', s']}$}
\\
\\ \tab \code{$\mathtt{y_{i\_fil}^{s}, y_{i,nn\_fil}^{s} = select\_top\,\left(y_{i}^{s},\,y_{i,nn}^{s}, \gamma\right)}$}
\\ 
\\ \tab \code{location\_cost = cos($\mathtt{y_{i\_fil}^{s}, y_{i,nn\_fil}^{s}}$)}
\\
\\ \tab \com{\# featured-based local cost}
\\ \tab \code{$\mathtt{y_{i,nn}^{s} = torch.zeros\_like(y_{i}^{s})}$}
\\
\tab \code{for r, s in R, S:}
\\
\tab \tab \code{r', s' = argmin($\mathtt{\left(L_2(y_{i}^{s}[r, s],\ y_{a}^{t}[r',s']\right)}$)}
\\
\tab \tab \code{$\mathtt{y_{i,nn}^{s}[r, s] = y_{a}^{t}[r', s']}$}
\\
\\ \tab \code{$\mathtt{y_{i\_fil}^{s}, y_{i,nn\_fil}^{s} = select\_top\,\left(y_{i}^{s},\,y_{i,nn}^{s}, \gamma\right)}$}
\\
\\ \tab \code{feature\_cost = cos($\mathtt{y_{i\_fil}^{s}, y_{i,nn\_fil}^{s}}$)}
\\
\\ \tab \code{\textbf{return} 0.5*(location\_cost + feature\_cost)}
\\ \rule{\textwidth}{0.5pt}
\\ \linebreak
We trained LVM-Med with graph size of $16$ nodes, each node connected to the top 5 nearest neighbors after using kNN, $\lambda$ value in Algorithm 1 is $80$, and $\alpha = 0.8$ for associating global- and local-based similarities when computing $c^{v}_{ij}$. The size of projector $h_{\phi}$ is $2048 \times 128$ for ResNet-50, and $768 \times 128$ for ViT. We configure the message passing network $g_{\theta}$ with two convolutional layers of size $128$. For the user-based prompt version, because the SAM model \cite{ma2023segment} requires an input of shape $256 \times 14 \times 14$ for the mask decoder part, we add two additional convolutional layers with a kernel size of $1$ and $3$ at the end of ViT backbone to convert from shape $768 \times 14 \times 14$ to the target shape. 
\section{Downstream task setups}
\label{sec:pre-downs-settings}
% \subsection{Pre-training}
% We trained LVM-Med with graph size of $16$ nodes, each node connected to the top 5 nearest neighbors after using kNN, $\lambda$ value in Algorithm 1 is $80$, and $\alpha = 0.8$ for associating global- and local-based similarities when computing $c^{v}_{ij}$. The size of projector $h_{\phi}$ is $2048 \times 128$ for ResNet-50, and $768 \times 128$ for ViT. We configure the message passing network $g_{\theta}$ with two convolutional layers of size $128$. For the user-based prompt version, because the SAM model \cite{ma2023segment} requires an input of shape $256 \times 14 \times 14$ for the mask decoder part, we add two additional convolutional layers with a kernel size of $1$ and $3$ at the end of ViT backbone to convert from shape $768 \times 14 \times 14$ to the target shape. 

\subsection{Downstream tasks}
\paragraph{Segmentation tasks}
On 2D-based segmentation tasks, we employ U-Net architecture \cite{ronneberger2015u} and load ResNet-50 \cite{he2016deep} trained by self-supervised learning algorithms as network backbones. With foundation models, we use TransUnet \cite{chen2021transunet} and take pre-trained ViT models as the backbones. For the prompt-based segmentation, we follow the architecture of SAM \cite{kirillov2023segment} consisting of encoder, prompt, and mask decoder layers. We also fine-tune SAM where encoder and prompt networks are frozen, only learning decoder layers \cite{ma2023segment}. Our LVM-Med for prompt-based setting is similar to \cite{ma2023segment} except that we substitute SAM's encoders with our weights. We utilize Adam optimizer for all experiments and train architectures with Dice and Cross-Entropy loss \cite{jadon2020survey}. We also normalize the norm-2 of gradient values to stabilize the training step to maximize 1.
Table \ref{tab:setting_2DSegmentation} summarizes each dataset's learning rate, number of epochs, and image resolution.   

On 3D-based segmentations, we reformulate these tasks as 2D segmentation problems and make predictions on 2D slices taken from 3D volumes. Furthermore, we apply balance sampling to select equally 2D slices covering target regions and other 2D slices, not including the ground truth. Table \ref{tab:setting_3DSegmentation}
presents configurations used for 3D datasets; other settings are identical to 2D cases.
% Please add the following required packages to your document preamble:
% \usepackage{multirow}
\begin{table}[h!]
\centering
\caption{Configurations for training 2D segmentation tasks}
\vspace{0.1in}
\label{tab:setting_2DSegmentation}
\resizebox{1.0\columnwidth}{!}{
\begin{tabular}{l|l|l|l|l|l}
\toprule
\textbf{} & \textbf{ISIC-2018 (Skin Lesion)} & \textbf{JSRT (Lung X-ray)} & \textbf{KvaSir (Polyp)} & \textbf{Drive (Vessel)} & \textbf{BUID (Breast Cancer)} \\ \midrule
\multirow{3}{*}{\textbf{ResNet-50.}} 
& lr = $10^{-4}$,  epochs $35$  & lr = $10^{-3}$, epochs $50$ &  lr = $10^{-3}$, epochs $35$  & lr = $10^{-3}$, epochs $50$ & lr = $10^{-4}$,  epochs $50$ \\
&  shape $512\times 512$ &  shape $224\times 224$&  shape $224\times 224$ &  shape $224\times 224$ &   shape $256\times 256$\\
& batch size $16$ & batch size $32$ & batch size $64$ & batch size $16$ &  batch size $8$\\ \midrule
\multirow{3}{*}{\textbf{Foundation Model}} 
& lr = $10^{-4}$,  epochs $100$  & lr = $10^{-3}$, epochs $200$ &  lr = $10^{-3}$,  epochs $200$ & lr = $10^{-3}$, epochs $200$ & lr = $10^{-4}$, epochs $200$  \\
&  shape $512\times 512$ &  shape $224\times 224$&  shape $224\times 224$ &  shape $224\times 224$ &  shape $256\times 256$\\
& batch size $16$ & batch size $32$ & batch size $64$ & batch size $16$ &  batch size $8$ \\ \midrule
\multirow{3}{*}{\textbf{Prompt-based Seg.}} 
& lr = $10^{-4}$,  epochs $50$  & lr = $3\times 10^{-4}$, epochs $50$ &  lr = $3\times 10^{-4}$,  epochs $20$ & lr = $3\times 10^{-4}$, epochs $100$ & lr = $10^{-4}$,  epochs $20$ \\
&   shape $1024\times 1024$ &  shape $1024\times 1024$ &  shape $1024\times 1024$ &  shape $1024\times 1024$ &  shape $1024\times 1024$\\
& batch size $16$ & batch size $16$ & batch size $16$ & batch size $16$ &  batch size $16$ \\ 
% & & & & & \\
% & & & & & \\
% & & & & & \\
\bottomrule
\end{tabular}}
\end{table}

% Please add the following required packages to your document preamble:
% \usepackage{multirow}
\begin{table}[H]
\centering
\caption{Configurations for 3D-based-segmentation tasks}
\vspace{0.1in}
\label{tab:setting_3DSegmentation}
\resizebox{0.95\columnwidth}{!}{
\begin{tabular}{l|l|l|l|l}
\toprule
\textbf{} & \textbf{BraTS} & \textbf{MMWHS-CT} & \textbf{MMWHS-MRI} & \textbf{BMC} \\ \midrule
\multirow{3}{*}{\textbf{\small{ResNet50}}} 
 &  lr = $15\times10^{-4}$, epochs $20$ & lr = $10^{-3}$, epochs $20$ &  lr = $15\times 10^{-4}$, epochs $30$  &  lr = $10^{-3}$, epochs $30$  \\
 &  shape $224 \times 224$ &  shape $224 \times 224$ &  shape $224 \times 224$ & shape $224 \times 224$  \\
 & batch size $128$ & batch size $64$ & batch size $64$ & batch size $64$ \\ 
\midrule
\multirow{3}{*}{\textbf{\small{Foundation Model}}}  
&  lr = $10^{-4}$, epochs $100$ & lr = $10^{-4}$, epochs $100$ &  lr = $10^{-4}$, epochs $100$  &  lr = $10^{-4}$, epochs $100$  \\
 & shape $224 \times 224$ & shape $224 \times 224$ &  shape $224 \times 224$ & shape $224 \times 224$  \\
 & batch size $16$ & batch size $16$ & batch size $16$ & batch size $16$  \\ \midrule
\multirow{3}{*}{\textbf{\small{Prompt-based Seg.}}}  
&  lr = $3 \times 10^{-5}$, epochs $30$ &  lr = $5\times 10^{-5}$, epochs $30$ &  lr = $3\times 10^{-5}$, epochs $30$  & lr = $3\times 10^{-4}$, epochs $50$  \\
 & shape $1024 \times 1024$ & shape $1024 \times 1024$ &  shape $1024 \times 1024$ & shape $1024 \times 1024$  \\
 & batch size $16$ & batch size $16$ & batch size $16$ & batch size $16$ \\ \bottomrule
\end{tabular}}
\end{table}
\paragraph{Image classification tasks}
We take the feature embedding outputs of each architecture and build one fully connected layer to produce desired classes for image classification tasks. We freeze the encoder layers for the linear evaluation and only train the fully connected layer. For the fully-finetuning, the whole network is trained. The Adam optimizer \cite{kingma2014adam} with cross-entropy loss function and learning rates $\{5\times 10^{-4}, 10^{-3}\}$ are used for Brain Tumor and FGADR, respectively. To benchmark LVM-Med with other state-of-the-art methods on FGADR (Figure 3 in paper), we follow the settings of DRG-Net \cite{tusfiqur2022drg} and change their encoder layers by our networks.  

\paragraph{Object detection}
We use Faster-RCNN \cite{girshick2015fast} for object detection tasks. The ResNet-50 of Faster-RCNN is replaced by pre-trained weights. In the Vin-Dr dataset, there is a total of $14$ objects for, e.g., Aortic enlargement, Atelectasis, Calcification, etc. We use  image resolutions of $512 \times 512$, Adam solver, and learning rate $10^{-4}$ in $40$ epochs. In the Kvasir dataset for polyp detection, we also resize images to a fixed size of $512 \times 512$, employ 
the Adam optimizer with learning rate $2.5\times\mathrm{10}^{-4}$ and batch size $8$. 

\section{LVM-Med ablation studies }
\label{sec:ablation-lvm-med}
\subsection{Graph sizes and $\lambda$ in backpropagation}
We provide in Figure \ref{fig:graph-numbers} and Figure \ref{fig:lambda_solver} LVM-Med performance when changing the number of nodes in graph construction steps  $G^{s}, G^{t}$ and $\lambda = 80$ used in Algorithm 1 in the backpropagation step. The results are reported on the average Dice score of five 2D segmentation tasks and the average accuracy of two linear classifications on FGADR and Brain Tumor Classification. Figure \ref{fig:graph-numbers} indicates that $16$ is the best value for both classification and segmentation. Increasing the graph's nodes tends to decrease classification performance. 

Figure \ref{fig:lambda_solver} compared different values for $\lambda \in \{70, 80, 90, 100\}$. We observe that $\lambda = \{80, 90\}$ achieve good results for linear classification tasks though $\lambda = \{90, 100\}$ decreases segmentation performance. 

\subsection{Performance on large- and small-scale}
We investigate LVM-Med performance when reducing the number of datasets in the pre-training step. Especially, we trained LVM-Med on a \textit{small-scale} with four datasets: LUNA2016~\cite{setio2015automatic}, LiTS2017~\cite{bilic2019liver}, BraTS2018~\cite{bakas2018identifying}, and MSD (Heart) \cite{simpson2019large}.  We compare this version with our default settings trained on $55$ datasets (Section \ref{sec:dataset_overview}). Two models are evaluated on dice scores of five 2D segmentation tasks, the accuracy metric of two linear image classifications, and mAP50 of two object detection tasks on VinDr and Kvasir detection. Table \ref{tab:ablation-study-2} shows that LMV-Med full leads to better performance overall, especially with the classification settings; the improvement gap is around $3.6\%$. In summary, we conclude that LVM-Med is beneficial when training in large-scale medical settings.

\begin{minipage}{\textwidth}
  \begin{minipage}[t]{0.48\textwidth}
    \begin{figure}[H]
\centering
\includegraphics[width=\textwidth]{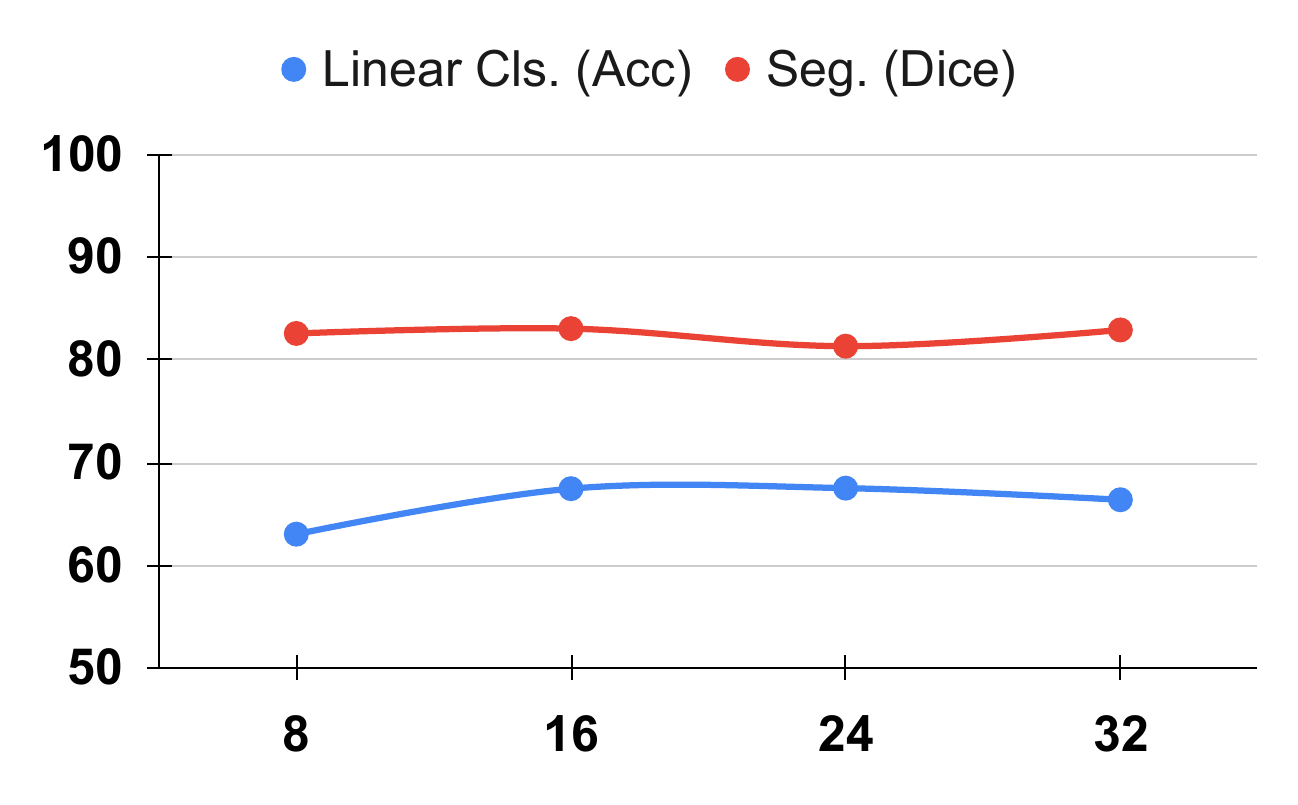}
\caption{\small{LVM-Med performance when varying the number of nodes in graph construction.}}
\label{fig:graph-numbers}
\end{figure}
  \end{minipage}
  \hfill
  \begin{minipage}[t]{0.48\textwidth}
    \begin{figure}[H]
\centering
\includegraphics[width=\textwidth]{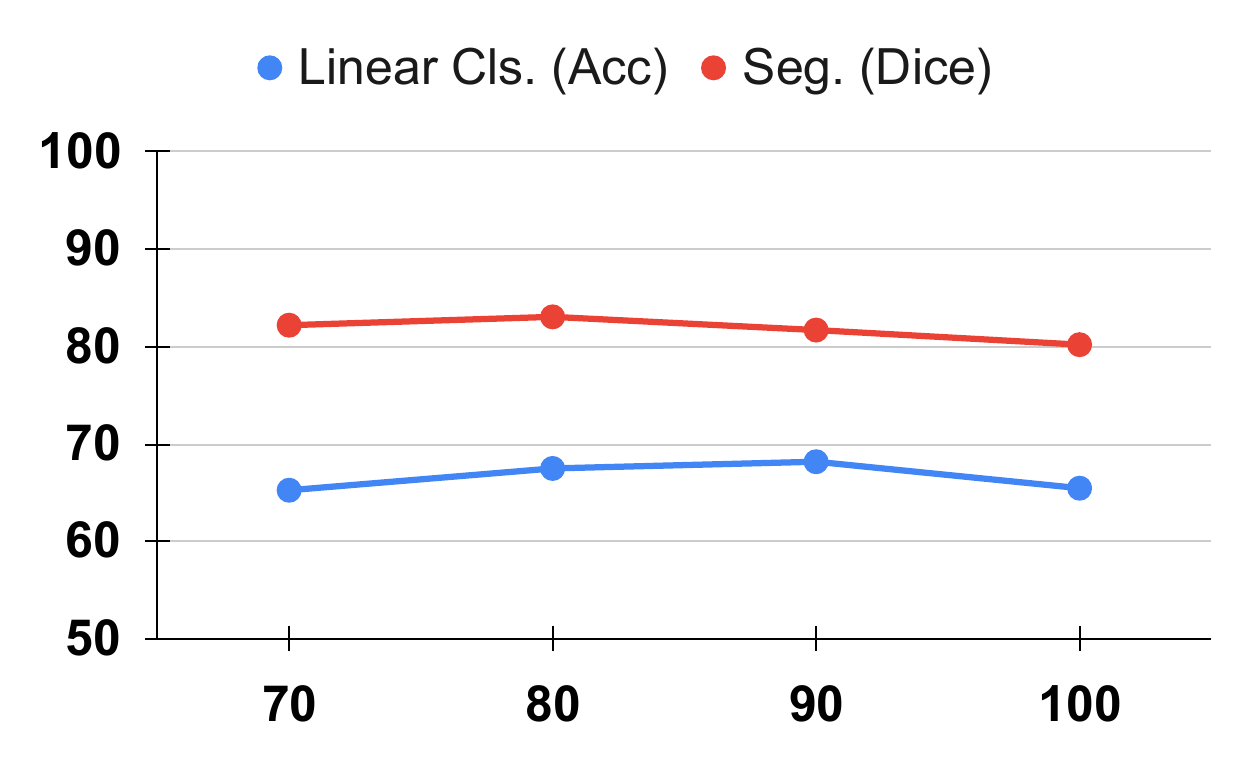}
\caption{\small{LVM-Med performance when varying the $\lambda$ in backpropagation step.}}
\label{fig:lambda_solver}
\end{figure}
  \end{minipage}
\end{minipage}

\subsection{Performance on weighting global and local similarities}
We test with different $\alpha = \{0.7, 0.8, 0.9\}$ which used to fuse global- and local-based similarities $c^{v}_{ij}$. Table \ref{tab:ablation-study-2} demonstrates that $\alpha = 0.8$ is generally the best value in average across segmentation, classification, and object detection tasks.

\begin{table}[H]
\centering
\caption{{LVM-Med ablation studies trained with full data, small-scale, and different hyper-parameter $\alpha$ fusing global- and local-based similarities. Results are reported on an average of five 2D segmentation, two linear classifications, and two object detection tasks. The most impacted factors are highlighted.}}
\label{tab:ablation-study-2}
\vspace{2mm}
\resizebox{0.8\columnwidth}{!}{
\begin{tabular}{ @{\hspace{-0pt}}l@{\hspace{8pt}}c@{\hspace{8pt}}c@{\hspace{10pt}}c}%rrrrrrrrrrrr
\toprule
Method         & Cls.(Acc)  & Seg. (Dice) & Detect. (mAP50)\\
\midrule
LVM-Med (full, $\alpha = 0.8$)                    & \textbf{67.47}     & \textbf{83.05}  & {57.1} \\
\rowcolor{cyan!50}
LVM-Med (small-scale, $\alpha = 0.8$)                   &  63.83  & 81.97  & 56.03  \\
LVM-Med (full, $\alpha = 0.7$)         & 65.89    & 82.20 & 56.49  \\
\rowcolor{cyan!50}
LVM-Med (full, $\alpha = 0.9$)            &  65.03   & 81.09 & \textbf{57.14} \\
\bottomrule
\end{tabular}}
\end{table}

\subsection{Computational complexity}
% We provide a parameter comparison of LVM-Med with other foundation models in Table \ref{tab:num-params}. Our LVM-Med with ResNet-50 version has a total of parameters approximately 3-4 times smaller than models like Flava or SAM but still maintains competitive performance. With LMV-Med using ViT encoder pre-trained by the SAM method, our parameter is approximate Flava model and is higher than Align $1.43$ times. However, it is important to note that both LVM-Med and SAM overall surpass these models with large margins.
We present a parameter comparison of LVM-Med with other foundation models in Table \ref{tab:num-params}. Our LVM-Med model, based on ResNet-50, has significantly fewer parameters, approximately 3-4 times smaller than models such as Flava or SAM, while still maintaining competitive performance. When utilizing the ViT encoder pre-trained by the SAM method, LVM-Med's parameters are comparable to the Flava model and slightly higher than Clip and Align by $1.03$ and $1.43$ times, respectively. However, it is important to note that both LVM-Med and SAM outperform these models by a significant margin in various settings.

\begin{table}[H]
\centering
\caption{{Computational complexity of our approaches and other foundation models.}}
\label{tab:num-params}
\vspace{2mm}
\resizebox{0.95\columnwidth}{!}{
\begin{tabular}{ @{\hspace{-0pt}}l@{\hspace{10pt}}c@{\hspace{10pt}}c@{\hspace{10pt}}c@{\hspace{10pt}}c@{\hspace{10pt}}c@{\hspace{10pt}}c}%rrrrrrrrrrrr
\toprule
Method         & LVM-Med (R50)  & LVM-Med (ViT)  & Clip \citep{radford2021learning} & Flava \citep{singh2022flava} & Align \citep{jia2021scaling} & SAM (Encoder) \citep{kirillov2023segment}\\
\midrule
\textbf{\#Param}   
& 25.55\,M     & 88.88\,M   & 85.80\,M  & 86.39\,M  & 62.14\,M  & 88.88\,M \\
\bottomrule
\end{tabular}}
\end{table}

\section{Prompt-based segmentation on 3D datasets and classification tasks}
\label{sec:linear-seg}
We provide additional results for LVM-Med on 3D-based prompt segmentation and image classification tasks with several fully connected layers. 
\subsection{Promt-based Segmentation on 3D datasets}
We perform experiments on three 3D datasets in Table \ref{tab:prompt-3Dsegmentation}, including BraTS, MMWHS-MRI, and MMWHS-CT. The setup for box prompts follows 2D segmentation cases. We discover that the LMV-Med in 3D cases consistently improves the performance of fine-tuned SAM \cite{ma2023segment} as in 2D settings and attains a large margin compared with SAM without training \cite{kirillov2023segment}. This evidence thus confirms that LVM-Med is also effective under prompt-based scenarios.

\begin{table}[H]
\centering
\caption{Prompt-based segmentation on 3D datasets.}
\vspace{0.1in}
\label{tab:prompt-3Dsegmentation}
\resizebox{1.0\columnwidth}{!}{
\begin{tabular}{l|l|ccc}
\toprule
 & \textbf{Method}              & \textbf{BraTS} & \textbf{MMWHS-MRI} & \textbf{MMWHS-CT} \\ \midrule
\multirow{3}{*}{\textbf{Prompt-based Seg.}} & SAM (fixed encoder) \citep{ma2023segment}& 85.37 $\pm$ 0.07 & 77.64 $\pm$ 1.14 & 76.61 $\pm$ 1.91 \\
 & SAM with Prompt (no-train) \citep{kirillov2023segment}  & 38.97 $\pm$ 0.21  & 59.74 $\pm$ 0.76      & 50.25 $\pm$ 0.33     \\
 & \textbf{LVM-Med (SAM's ViT)} &    \textbf{85.76 $\pm$0.07}            & \textbf{78.91 $\pm$ 0.80}      & \textbf{78.03 $\pm$ 0.93}     \\ \bottomrule
\end{tabular}}
\end{table}

\subsection{Image classification}
We aim to inspect whether foundation models improve their performance given more fully connected layers for image classification tasks with both frozen encoders or fully fine-tuning.
For each method in this category and our LVM-Med (ResNet-50 and ViT), we configure two fully connected layers with sizes $512-256$ and $512-128$ for the Brain and FGADR respectively that map from the output dimension of each network to a number of desired classes. Table \ref{tab:linear-classification} presents obtained results where new settings are highlighted in color. We notice the following points. (i) Firstly, using more fully connected layers tends to improve the performance of foundation models, especially on linear evaluation. For e.g., the Clip increases from $4.79\%-9.98\%$ on FGADR and Brain Tumor classification tasks, respectively. Similarly, our LVM-Med with SAM's ViT also achieves better results by approximately  $1.37\%$ and $4.82\%$ on those tasks. (ii) Secondly, LVM-Med overall  attains the best results in four settings using linear or several fully connected layers with ResNet-50. LVM-Med with ViT architecture also delivers the best records on three of four test cases compared with foundation models. 

\begin{table}[!t]
\begin{center}
\caption{\small{Comparing SSL approaches and Foundation models on classification tasks with two evaluation protocols, Linear evaluation and full Fine-tuning. Settings used with several fully connected layers are in cyan. The best results in 2D-SSL and foundation models (two fully connected layers) are in bold; the best results overall are in bold and underlined.}}
\vspace{0.1in}
\label{tab:linear-classification}
\resizebox{\columnwidth}{!}{
\begin{tabular}{l|l|cccc}
\toprule
\textit{} &
  \textbf{Method} &
  \multicolumn{2}{c}{\textbf{Linear Evaluation (Frozen)}} &
  \multicolumn{2}{c}{\textbf{Fine-tuning}} \\ \midrule
\textit{} &
   &
  \textbf{FGADR (DR Grading)} &
  \textbf{Brain Tumor Class.} &
  \textbf{FGADR (DR Grading)} &
  \textbf{Brain Tumor Class.} \\ \midrule
\multirow{8}{*}{\textbf{2D-SSL on medical}} &
  Twin-Barlon \cite{zbontar2021barlow}&
  {66.86 $\pm$ 0.41} &
  63.03 $\pm$ 0.32 &
  {66.37 $\pm$ 0.77} &
  74.20 $\pm$ 1.38 \\
 &
  Dino \cite{caron2021emerging}&
  65.98 $\pm$ 1.91 &
  62.27 $\pm$ 0.32 &
  67.35 $\pm$ 1.36 &
  71.91 $\pm$ 1.55 \\
 &
  SimCLR \cite{chen2020simple}&
  65.30 $\pm$ 1.70 &
  62.52 $\pm$ 1.67 &
  67.55 $\pm$ 0.28 &
  73.52 $\pm$ 3.56 \\
 &
  Moco-v2 \citep{chen2020improved}&
  65.98 $\pm$ 1.04 &
  62.35 $\pm$ 1.92 &
  67.55 $\pm$ 1.79 &
  74.53 $\pm$ 0.43 \\
 &
  Deepcluster \citep{caron2018deep}&
  65.34 $\pm$ 1.93 &
  {64.47 $\pm$ 0.55} &
  67.94 $\pm$ 1.78 &
  73.10 $\pm$ 0.55 \\
 &
  VicRegl \citep{bardes2022vicregl}&
  64.71 $\pm$ 0.60 &
  59.64 $\pm$ 1.36 &
  65.69 $\pm$ 1.46 &
  73.18 $\pm$ 2.03 \\ 
 &
  \multirow{2}{*}{\textbf{LVM-Med (R50)}} &
  \textbf{\underline{68.33} $\pm$ 0.48} 
  & 66.33 $\pm$ 0.31
  & 68.32 $\pm$ 0.48
  & 76.82 $\pm$ 2.23  \\ 
  & & 
  \cellcolor{cyan!50}
  {{66.67} $\pm$ 0.84} &
  \cellcolor{cyan!50} \textbf{\underline{74.70} $\pm$ 0.84} &
  \cellcolor{cyan!50} \textbf{\underline{70.58} $\pm$ 0.36} &
  \cellcolor{cyan!50} \textbf{\underline{78.77} $\pm$ 0.78} \\ \midrule
\multirow{10}{*}{\textbf{Foundation Model}} &
  \multirow{2}{*}{Clip \citep{radford2021learning}} &
  57.87 $\pm$ 0.50  
  & 57.87 $\pm$ 0.71
  & 57.48 $\pm$ 0.86
  & 34.86 $\pm$ 2.27 \\
  & &
  % \rowcolor{cyan!50} 
  \cellcolor{cyan!50}62.66 $\pm$ 0.36 &
  \cellcolor{cyan!50}\textbf{67.85 $\pm$ 0.23} &
  \cellcolor{cyan!50}56.21 $\pm$ 1.86 &
  \cellcolor{cyan!50}21.74 $\pm$ 1.14 \\ \cmidrule{2-6}
 &
  \multirow{2}{*}{Flava \citep{singh2022flava}} &
  31.87 $\pm$ 0.69 
  & 35.19 $\pm$ 0.43
  & 57.18 $\pm$ 0.96
  & 34.01 $\pm$ 5.97 \\
  & &
  % \rowcolor{cyan!50}
  \cellcolor{cyan!50}32.84 $\pm$ 0.12  &
 \cellcolor{cyan!50} 24.45 $\pm$ 4.30 &
  \cellcolor{cyan!50}{56.01 $\pm$ 0.86} &
  \cellcolor{cyan!50} 33.67 $\pm$ 8.11  \\ \cmidrule{2-6}
 &
  \multirow{2}{*}{Algin \citep{jia2021scaling}} &
  36.95 $\pm$ 1.04 
  & 30.71 $\pm$ 2.35
  & 57.28 $\pm$ 0.97
  & 63.96 $\pm$ 0.04 \\ 
  & &
   % \rowcolor{cyan!50}
   \cellcolor{cyan!50}38.12 $\pm$ 1.45 &
 \cellcolor{cyan!50} 30.34 $\pm$ 1.35 &
  \cellcolor{cyan!50}57.87 $\pm$ 0.90 &
  \cellcolor{cyan!50}61.42 $\pm$ 0.25 \\ \cmidrule{2-6}
 &
  \multirow{2}{*}{SAM \citep{kirillov2023segment}} &
  55.13 $\pm$ 0.41 
  & 31.81 $\pm$ 4.26
  & 58.75 $\pm$ 1.32
  & 60.66 $\pm$ 1.36 \\
  & &
  % \rowcolor{cyan!50}
  \cellcolor{cyan!50}57.48 $\pm$ 0.24 &
  \cellcolor{cyan!50} 36.89 $\pm$ 1.61 &
  \cellcolor{cyan!50} 58.75 $\pm$ 0.99 &
  \cellcolor{cyan!50} 60.07 $\pm$ 0.31 \\ \cmidrule{2-6}
 &
  \multirow{2}{*}{\textbf{LVM-Med (SAM's ViT)}} &
  62.46 $\pm$ 0.86 
  & 59.31 $\pm$ 0.48
  & 63.44 $\pm$ 0.73
  & 67.34 $\pm$ 2.08\\ 
  & &
  % \rowcolor{cyan!50} 
  \cellcolor{cyan!50}\textbf{63.83 $\pm$ 1.36} &
  \cellcolor{cyan!50}64.13 $\pm$ 1.14 &
  \cellcolor{cyan!50}\textbf{59.04 $\pm$ 0.14} &
  \cellcolor{cyan!50}\textbf{64.97 $\pm$ 2.71} \\ \bottomrule
\end{tabular}}
\end{center}
\end{table}

\section{Visualizing results}
We provide qualitative results for prompt-based segmentation in Figure \ref{fig:SAM_demo}. We compare three approaches, including (i) the standard SAM without fine-tuning \cite{kirillov2023segment} (second column), (ii) SAM with encoders and prompt networks are frozen, and only decoder layers are trained as  \cite{mazurowski2023segment} (third column), and (iii) a similar setting as (ii) but encoders taken from LVM-Med version with SAM's ViT architecture (fourth column). For all methods, we simulate box-based prompts using the ground-truth masks and define boxes covering those target regions perturbed by offset values. 

Figure \ref{fig:SAM_demo} demonstrates that the original SAM is prone to generate useless predictions (top and bottom rows) or less precise boundaries. In contrast, updated SAM and LVM-Med produce more accurate results, confirming the importance of fine-tuning to achieve adequate results. Figures in the third and fourth columns also illustrate that SAM tends to over-segment or lacks structures on an object's edges in several cases, while LVM-Med is more stable in those situations (red arrows). 
\label{sec:visualize_images}

\begin{figure}[H]
    \centering
    \fontsize{26pt}{26pt}\selectfont
    \resizebox{1.0\columnwidth}{!}{
    \begin{tabular}{cccc}
    \includegraphics[width=10cm]{Figs/SAM_demo/malignant(120)_groundtruth.png} &
      \includegraphics[width=10cm]{Figs/SAM_demo/malignant(120)_nofinetune.png} &
      \includegraphics[width=10cm]{Figs/SAM_demo/malignant(120)_finetune.png}  &
      \includegraphics[width=10cm]{Figs/SAM_demo/malignant(120)_our.png}  \\
      
      \includegraphics[width=10cm]{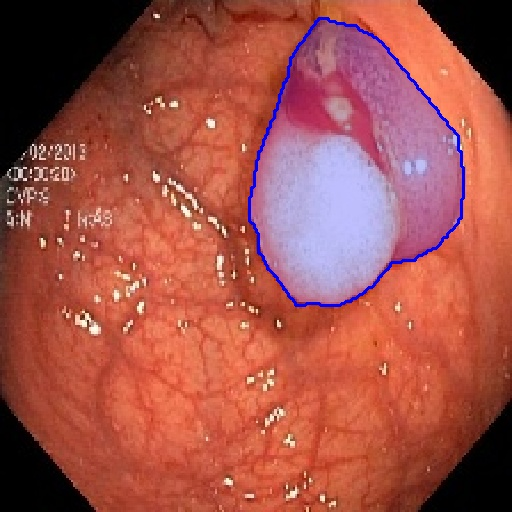} &
      \includegraphics[width=10cm]{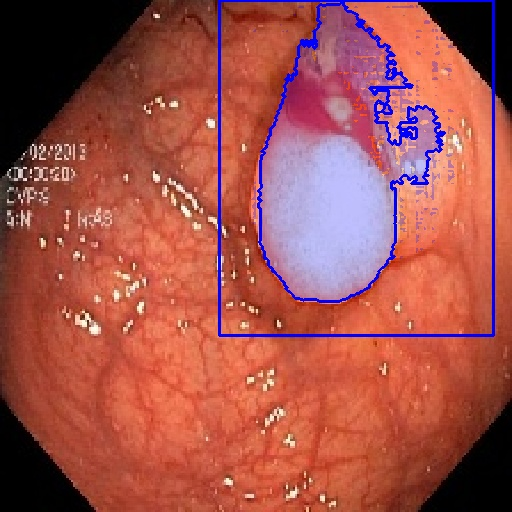} &
      \includegraphics[width=10cm]{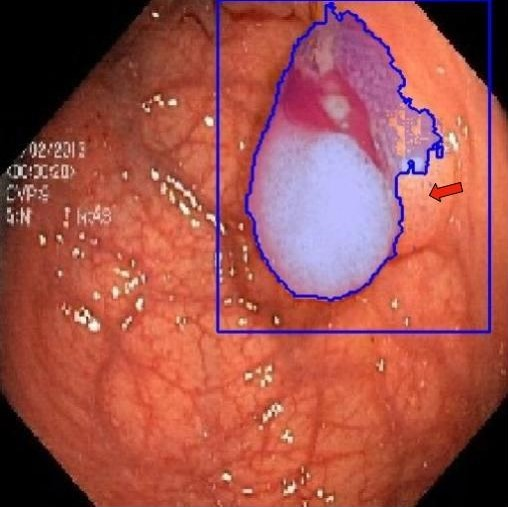}  &
      \includegraphics[width=10cm]{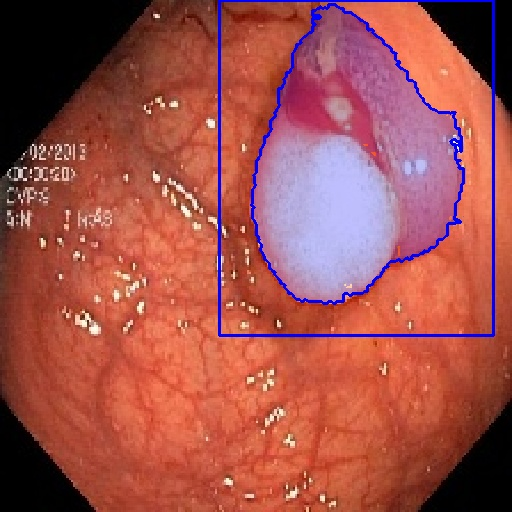}  \\

    \includegraphics[width=10cm]{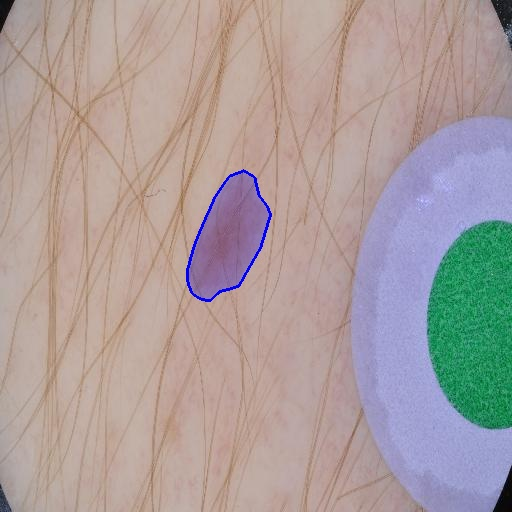} &
      \includegraphics[width=10cm]{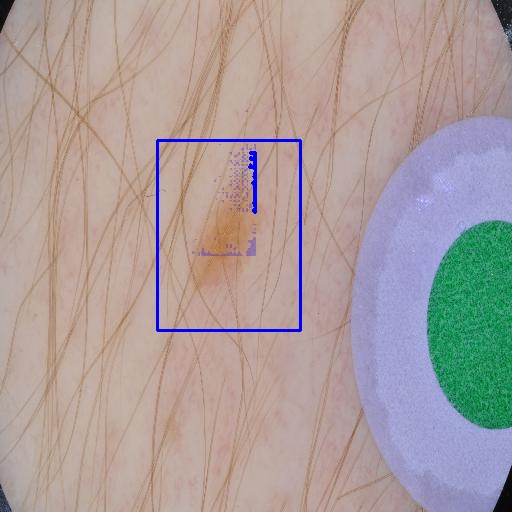} &
      \includegraphics[width=10cm]{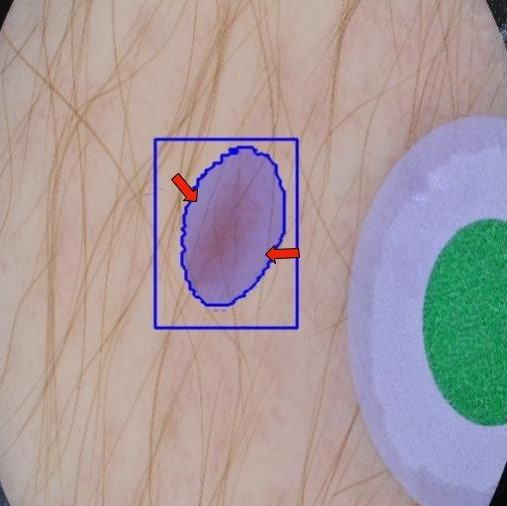}  &
      \includegraphics[width=10cm]{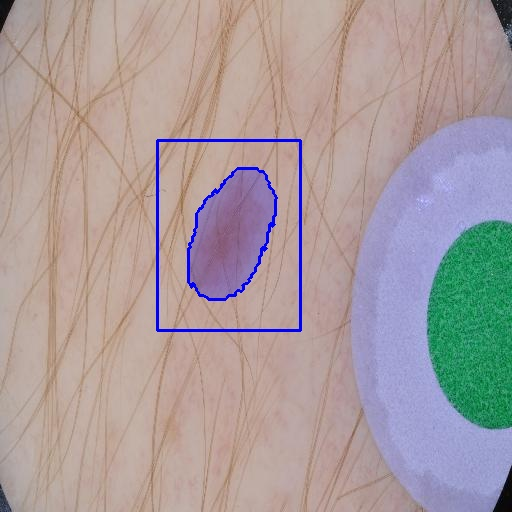}  \\
       
      Ground Truth &
      SAM (no fine-tuning) \cite{kirillov2023segment} &
      SAM (fine-tuning) \cite{ma2023segment}&
      LVM-Med (SAM's ViT)  \\      
    \end{tabular}}    
    \caption{Visualizing prompt-based predictions on three datasets: BUID, Kvasir, and ISIC. Red arrows show differences between SAM (fine-tuning) and LVM-Med using SAM's ViT architecture. Best viewed in color with \textbf{zoom}.}
    \label{fig:SAM_demo}
\end{figure}

\section{Dataset overviews}
\label{sec:dataset_overview}
Table \ref{tab:data1} overviews the dataset used in our study. For each dataset, we provide its modality, data dimension, and the total of samples. If the training/testing rate is available (column \textbf{Train/Test Rate}), we utilize all training data; otherwise, we sample $20\%$ total samples to avoid potential test data leaking for downstream tasks used in the pre-training  step. For datasets whose data dimensions are  3D volumes, we sample 2D slices from those formats. Some datasets, such as MSD or ADNI, comprise different sub-datasets inside; we consider these sub-sets as independent ones to avoid confusion during the training steps. In summary, a total of $55$ datasets are used with approximately $40\%$ in 3D datasets and $60\%$ in 2D images as presented in Figure \ref{fig:3d-2d-ration}. Moreover, we also outline ratios between distinct data modalities such as MRI, CT, X-ray, grayscale types such as Ultrasound, OCT, and finally, color images depicted in Figure \ref{fig:modularity-ratio}.
\vspace{-0.3in}
\begin{minipage}{\textwidth}
  \begin{minipage}[t]{0.48\textwidth}
    \begin{figure}[H]
\centering
\includegraphics[width=\textwidth]{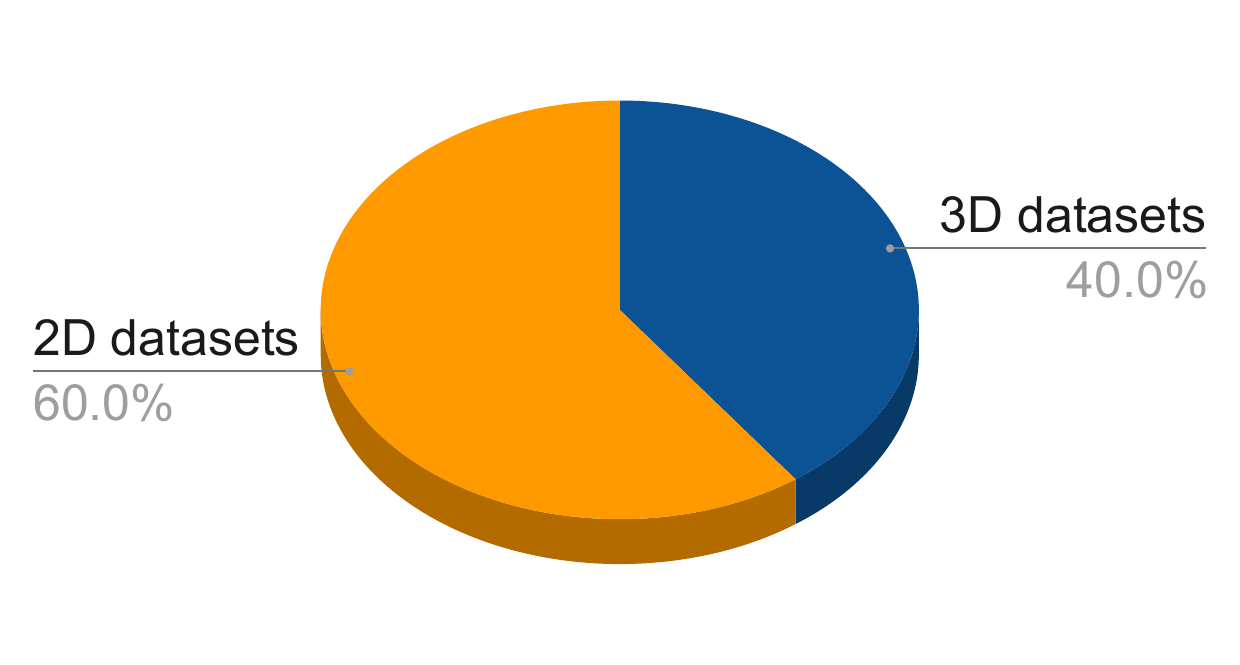}
\caption{\small{Pie chart illustrating the ratio of the number of datasets with the 3D  and 2D dimension.}}
\label{fig:3d-2d-ration}
\end{figure}
  \end{minipage}
  \hfill
  \begin{minipage}[t]{0.48\textwidth}
    \begin{figure}[H]
\centering
\includegraphics[width=\textwidth]{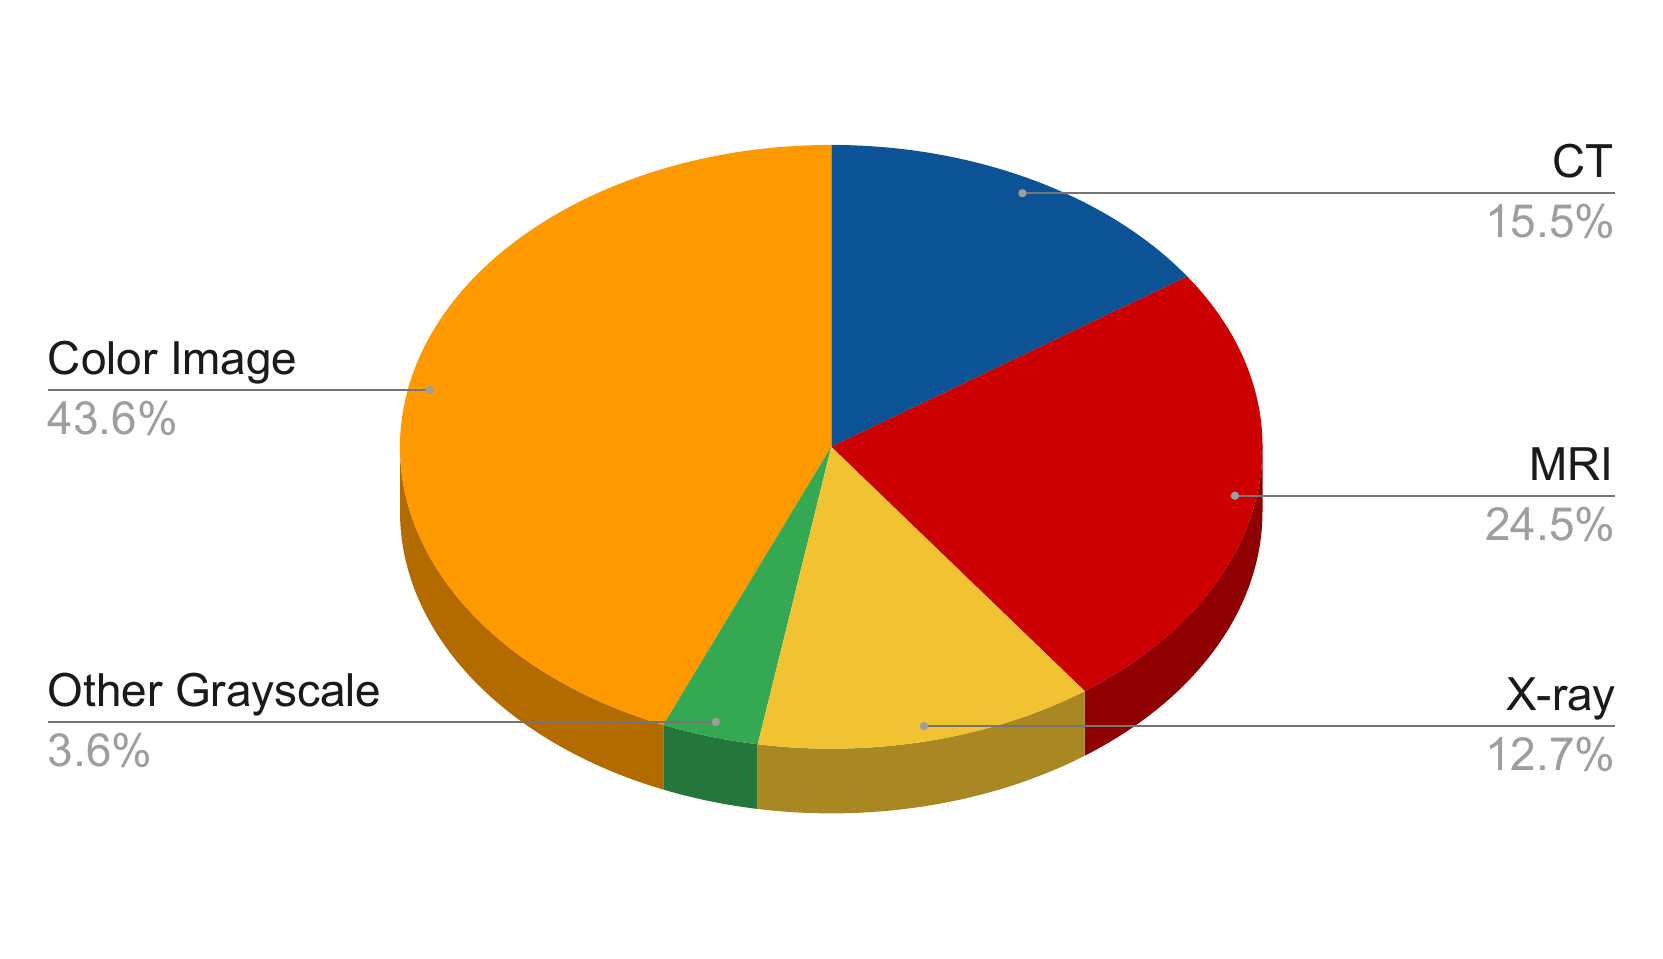}
\caption{\small{Pie chart illustrating the ratio of different data modalities in our collected dataset.}}
\label{fig:modularity-ratio}
\end{figure}
  \end{minipage}
\end{minipage}

\begin{table}[H]
\caption{Overview of our collected medical dataset}
\vspace{2mm}
\centering
\resizebox{1.0\columnwidth}{!}{
\begin{tabular}{p{1cm}p{2cm}p{2cm}p{3cm}p{1.2cm}p{1.5cm}p{1.23cm}p{1cm}}
\toprule
\textbf{No}&\textbf{Data Name}&\textbf{Topic}&\textbf{Disease}&\textbf{Modality}&\textbf{Dimension}&\textbf{Train/Test Rate?}&\textbf{Total}\\ \midrule
1&HyperKvasir \cite{borgli2020hyperkvasir}&Polyp&Pathological classification&Color images&2D&Yes&110079\\\midrule
2&PatchCamelyon \cite{Veeling2018-qh, bejnordi2017diagnostic}&Cells&Histopathologic scans of lymph node sections.&Color images&2D&Yes&327680\\\midrule
3&BraTS2018 \cite{6975210, lloyd2017high, bakas2018identifying}&Brain&Tumor Segmentation&MRI&3D&No&760\\\midrule
4&HNSCC \cite{grossberg2018imaging} &Head Neck&No Label&CT&3D&No&155\\\midrule
5&LiTS2017 \cite{bilic2023liver}&Liver&Segmentation of Liver and Tumor Lesions&CT&3D&No&200\\\midrule
6&MSD-Heart \cite{simpson2019large}&Heart&Heart Segmentation&MRI&3D&No&30\\\midrule
7&MSD-Liver \cite{simpson2019large}&Liver&Liver Segmentation&MRI&3D&No&201\\\midrule
8&MSD-Lung \cite{simpson2019large}&Lung&Lung Segmentation&MRI&3D&No&96\\\midrule
9&MSD-Pancreas \cite{simpson2019large}&Pancreas&Pancrea Segmentation&MRI&3D&No&420\\\midrule
10&MSD-HepaticVessel \cite{simpson2019large}&Hepatic Vessel &Hepatic Vessel Segmentation&MRI&3D&No& 443\\\midrule
11&MSD-Spleen \cite{simpson2019large}&Spleen&Spleen Segmentation&MRI&3D&No& 61\\\midrule
12&MSD-Colon \cite{simpson2019large}&Colon&Colon Segmentation&MRI&3D&No&190\\\midrule
13&OPC-Radiomics \cite{kwan2018radiomic,clark2013cancer, kwandata}&Oropharynx&No Label&CT&3D&No&120\\\midrule
14&Osteosarcoma-UT \cite{leavey2019osteosarcoma,yorke2019pelvic, clark2013cancer}&Osteosarcoma&No Label&Color images&2D&No&547\\ \midrule
15&Pancreas-CT \cite{roth2016data, roth2015deeporgan, clark2013cancer}&Pancreas&No Label&CT&3D&No&16\\\bottomrule
\end{tabular}}
\vspace{1mm}
% and the effectiveness of two arbitrary style transfers, AdaIN and EFDM
\label{tab:data1}
\end{table} 

% \begin{landscape}
\begin{table}[H]
\centering
\resizebox{1.0\columnwidth}{!}{
\begin{tabular}{p{1cm}p{2cm}p{2cm}p{3cm}p{1.2cm}p{1cm}p{1.23cm}p{1cm}}
\toprule
\textbf{No}&\textbf{Data Name}&\textbf{Topic}&\textbf{Disease}&\textbf{Modality}&\textbf{Format}&\textbf{Default Train/Test Rate}&\textbf{Total}\\ \toprule
16&Pelvic-Reference-Data \cite{yorke2019pelvic, clark2013cancer}&Pelvic&No Label&CT&3D&No&12\\\midrule
17&ProstateX \cite{litjens2014computer, Litjens2017, clark2013cancer}&Prostate&The clinical significance of prostate lesions prediction&MRI&3D&No&40\\\midrule
18&TCGA-CESC \cite{lucchesi2016radiology, clark2013cancer}&Cervical&No Label&Color images&2D&No&3977\\\midrule
19&TCGA-COAD \cite{kirk2016radiology, clark2013cancer}&Colon&No Label&Color images&2D&No&1644\\\midrule
20&TCGA-ESCA \cite{Lucchesi20164, clark2013cancer}&Cuticle&No Label&Color images&2D&No&4427\\\midrule
21&TCGA-KICH \cite{linehan2016radiology, clark2013cancer}&Kidney&No Label&Color images&2D&No&2192\\\midrule
22&TCGA-KIRC \cite{akin2016radiology, clark2013cancer}&Kidney&No Label&Color images&2D&No&34108\\\midrule
23&TCGA-READ \cite{kirk2016radiology, clark2013cancer}&Rectum&No Label&Color images&2D&No&248\\\midrule
24&TCGA-SARC \cite{roche2016radiology, clark2013cancer}&Sarcoma&No Label&Color images&2D&No&624\\\midrule
25&TCGA-THCA \cite{kirk2016radiology, clark2013cancer}&Thyroid&No Label&Color images&2D&No&665\\\midrule
26&VinDr \citep{nguyen2022vindr}&Lung&Abnormal Disease Classification&X-ray&2D&No&18000\\\midrule
27&LUNA2016 \cite{setio2015automatic}&Lung&Nodule Detection and False Positive Reduction&CT&3D&No&49386\\\midrule
28&BCCD \cite{BCCD_Dataset}&Cells&Blood cell detection&Color images&2D&No&364\\ \midrule
29&C-NMC\_Leukemia \cite{gehlot2020sdct, gupta2019all}&Cells&Leukemia detection&Color images&2D&Yes&12529\\ \midrule
30&CBIS-DDSM \cite{lee2017curated, sawyer2016curated}&Breast&Breast Cancer Classification&X-ray&2D&No&6774\\\midrule
31&COVIDx \cite{Wang2020}&Lung&Covid-19 Detection&X-ray&2D&Yes&194922\\\midrule
32&Heidelberg OCT \cite{kermany2018labeled}&Eye&OCT Imaging Classification&OCT&2D&Yes&84495\\\midrule
33 &m2caiSeg \cite{maqbool2020m2caiseg}&Laparoscopic&Semantic Segmentation Laparoscopic&Color images&2D&Yes&614\\\midrule
34&NuCLS \cite{amgad2102nucls}&Nucleus&Nucleus Segmentation Detection / Classification&Color images&2D&Yes&1744\\\midrule
35&SARAS-MESAD \cite{cuzzolin2021saras}\cite{saras-mesad2}\cite{saras-mesad3}&Prostatectomy Procedures&Action classification in Prostatectomy Surgey&Color images&2D&Yes&29454\\\midrule
36&Shoulder X-ray images from Sun Yat-sen Memorial Hospital \cite{shoulder}&Shoulder&Shoulder X-ray Classification&X-ray&2D&Yes&1049\\\bottomrule
\end{tabular}}
\vspace{1mm}
%\caption{Overview our collected medical dataset}
% and the effectiveness of two arbitrary style transfers, AdaIN and EFDM
\label{tab:data2}
\end{table}

\begin{table}[H]
\centering
\resizebox{1.0\columnwidth}{!}{
\begin{tabular}{p{1cm}p{2cm}p{2cm}p{3cm}p{1.2cm}p{1cm}p{1.23cm}p{1cm}}
\toprule
\textbf{No}&\textbf{Data Name}&\textbf{Topic}&\textbf{Disease}&\textbf{Modality}&\textbf{Format}&\textbf{Default Train/Test Rate}&\textbf{Total}\\ \toprule
37&Shenzhen Hospital X-ray Set \cite{ShenzhenHospitalX-raySet}&Lung&Lung segmentation&X-ray&2D&No&566\\\midrule
38&ADNI 1.5T  \cite{mueller2005alzheimer,petersen2010alzheimer}&Brain&Alzheimer's Disease Classification&MRI&3D&No&639\\\midrule
39&ADNI 3T \cite{mueller2005alzheimer,petersen2010alzheimer}&Brain&Alzheimer's Disease Classification&MRI&3D&No&119\\\midrule
40&AML-Cytomorphology \cite{matek2019single, matek2019human,clark2013cancer}&Cell&Peripheral blood smears&Color images&2D&No&18365\\\midrule
41&APTOS 2019 \cite{karthick2019aptos}&Eye&Severity of diabetic retinopathy Classification&Color images&2D&No&3662\\ \midrule
42&BCSS \cite{amgad2019structured}&Cells&Breast cancer semantic segmentation&Color images&2D&No&151\\\midrule
43&Dental Panoramic \cite{abdi2020panoramic}&Tooth&Mandible segmentation&X-ray&2D&No&116\\\midrule
44&HC18 \cite{van2018automated}&Fetal&Fetal head circumference (HC)&Ultrasound&2D&No&999\\\midrule
45&Hippseg 2011 \cite{Hippseg2011}&Brain&Hippocampus Segmentation&MRI&3D&No&3050\\\midrule
46&ISIC Challenge 2019 \cite{isic}&Skin&Skin Cancer Classification&Color images&2D&No&25331\\\midrule
47&KiTS19-21 \cite{taha2018kid}&Kidney&Kidney Segmentation&CT&3D&No&45424\\\midrule
48&Kvasir v2 \cite{kvarsir}&Gastrointestinal&Gastrointestinal cancer image classification&Color images&2D&No&6000\\\midrule
49&LHNCBC Malaria \cite{Malaria}&Cells&Malaria Classification&Color images&2D&No&27560\\\midrule
50&MitoEM \cite{wei2020mitoem}&Cells&Mitochondria Instance Segmentation&MRI/CT&3D&No&1000\\\midrule
51&MLL Bone Marrow \cite{matek2021highly}&Cells&Blood cell classification&Color images&2D&No&171374\\\midrule
52&MMWHS-CT\cite{zhuang2016multi}&Heart&Sub-structure Heart segmentation&CT&3D&Yes& 40\\\midrule
53&MMWHS-MRI \cite{zhuang2016multi}&Heart&Sub-structure Heart segmentation&MRI&3D&Yes& 40\\\midrule
54&RSNA Bone Age \cite{halabi2019rsna}&Bone&Bone age prediction&X-ray&2D&No&12611\\\midrule
55&EyePACS \cite{eyePACS} &Eye& Diabetic Retinopathy Detection&Color Images&2D&Yes&88702\\\bottomrule
\end{tabular}}
\vspace{2mm}
% and the effectiveness of two arbitrary style transfers, AdaIN and EFDM
\label{tab:data3}
\end{table} 

% Uncomment lines above for seperate file
% \clearpage
% \bibliography{references}
% \end{document}
